# Supplementary material for: Optimal Performance of Feedback Control Systems with Limited Communication over Noisy Channels
Source: arXiv:math/0609266 source file (2006-09-10)
Supplement: Supplementary file 1 [file appendix.tex]

\section{Proof of \autoref{thm:discounted}}
\label{app:discounted}
\begin{definition}
  Let $\V$ be the family of functions from 
  $\P{\X\times\M\times\P{\X\times\M}}$ to $\RR_+$ and let $\Gamma$ denote 
  $\sC\times\sL\times\sG_s$. For any $\gamma \in \Gamma$ define an operator 
  $H(\gamma)$ from $\V$ to $\V$ according to
  \begin{equation}
    \left( H(\gamma)V \right)(\pi) = \hat \rho(\gamma,\pi) + \beta 
    V(\widetilde Q(\gamma) \pi ) \quad \forall V \in \V,
  \end{equation}
  where $\hat \rho(\gamma,\pi) \defined \tilde \rho(\widehat Q(\gamma) \pi, 
  g)$, $\gamma = (c,g,l)$ and $\widetilde Q(\gamma) \defined \widetilde 
  Q(c,l,g)$ and $\widehat Q(\gamma) = \widehat Q(c,l)$ are defined 
  by~\eqref{eq:Qtilde} and~\eqref{eq:Qhat} respectively.
\end{definition}

\begin{definition}
  Define a transformation $\H$ from $\V$ to $\V$ according to
  \begin{equation}
    \big( \H V \big)(\pi) = \inf_{\gamma \in \Gamma} \big( H(\gamma)V 
    \big)(\pi).
  \end{equation}
\end{definition}

The system of \autoref{prob:beta} can be rewritten as follows. For any design 
$\gamma' \defined (\gamma'_1, \gamma'_2, \dots) \in \Gamma^\infty$,the state 
evolves according to
\begin{equation}
  \pi_{t+1} = \widetilde Q(\gamma'_t)\pi_t,
  \label{eq:beta_state}
\end{equation}
where the transformation $\widetilde Q$ is known. The expected discounted 
cost of any design $\gamma'$ is given by
\begin{equation}
  \J^\beta(\gamma') \defined \sum_{t=1}^{\infty} \beta^{t-1} \hat \rho(\pi_t, 
  \gamma'_t),
\end{equation}
The objective is to minimize $\J^\beta(\gamma')$ over all choices of 
$\gamma'$.

This is a classical deterministic infinite horizon discounted cost problem 
whose value function is given by the unique uniformly bounded fixed point of
\begin{equation}
  V(\pi) = \big(\H V\big)(\pi).
\end{equation}
An optimal stationary policy is given by $\gamma^\infty = 
(\gamma,\gamma,\cdots)$ where $\gamma$ satisfies
\begin{equation}
  V(\pi) = \big(H(\gamma)V\big)(\pi).
\end{equation}
This completes the proof of \autoref{thm:discounted}. \hfill \qed

\section{Proof of \autoref{thm:average}}
\label{app:avg}

Let $\widetilde Q, \hat \rho$ and $\Gamma$ be defined as in the proof of 
\autoref{thm:discounted} (Appendix~\ref{app:discounted}). Then the system of 
\autoref{prob:avg} can be rewritten as follows.  For any design $\gamma' 
\defined (\gamma'_1, \gamma'_2, \dots) \in \Gamma^\infty$,the state evolves 
according to
\begin{equation}
  \pi_{t+1} = \widetilde Q(\gamma'_t)\pi_t,
  \label{eq:avg_state}
\end{equation}
where the transformation $\widetilde Q$ is known. The expected discounted 
cost of any design $\gamma'$ is given by
\begin{equation}
  \overline{\J}(\gamma') \limsup_{T \to \infty} \frac 1T \sum_{t=1}^{T} \hat 
  \rho(\pi_t, \gamma'_t).
  \label{eq:avg_cost}
\end{equation}
The objective is to minimize $\overline{\J}(\gamma')$ over all choices of 
$\gamma'$. This is a classical deterministic average cost per unit time 
problem.  Conditions (A1) corresponds to the canonical form of this 
system~\cite[Chapter~7]{Dynkin:1975}. If a design $(\design[0])$ and 
measurable bounded functions $v(\cdot)$ and $r(\cdot)$ satisfy the canonical 
form, then the design is $\varepsilon$-optimal in the sense 
of~\eqref{eq:diff} and~\eqref{eq:avg_inf}~\cite[Chapter~7]{Dynkin:1975}.  
\hfill \qed
